# Supplementary material for: Observation of Beam Spin Asymmetries in the Process $e p \rightarrow e \pi^{+}\pi^{-}X$ with CLAS12
Source: arXiv:2101.04842 ancillary file (2021-03-27)
Supplement: Supplementary file 1 [file appendix.pdf]

**Ancillary files for “Observation of Beam Spin Asymmetries in the  
Process  $ep \rightarrow e'\pi^+\pi^-X$  with CLAS12”**

CLAS Collaboration

## I. BEAM SPIN ASYMMETRIES

The extracted asymmetry values for all seven azimuthal modulations in each bin are given in Tables I-VI. The listed asymmetry amplitudes have been corrected for the beam polarization and, if desired, can be further corrected for the relevant twist-2 or twist-3 kinematic depolarization factors defined in Refs [1–3],

$$K_2 \equiv \frac{C(\epsilon, y)}{A(\epsilon, y)}, \quad (1)$$

$$K_3 \equiv \frac{W(\epsilon, y)}{A(\epsilon, y)}, \quad (2)$$

with

$$A(\epsilon, y) \equiv \frac{y^2}{2(1-\epsilon)} = \frac{1}{1+\gamma^2} \left( 1 - y + \frac{1}{2}y^2 + \frac{1}{4}\gamma^2 y^2 \right), \quad (3)$$

$$C(\epsilon, y) \equiv \frac{y^2}{2(1-\epsilon)} \sqrt{1-\epsilon^2} = \frac{y}{\sqrt{1+\gamma^2}} \left( 1 - \frac{1}{2}y \right), \quad (4)$$

$$W(\epsilon, y) \equiv \frac{y^2}{2(1-\epsilon)} \sqrt{2\epsilon(1-\epsilon)} = \frac{y}{\sqrt{1+\gamma^2}} \sqrt{1 - y - \frac{1}{4}\gamma^2 y^2}. \quad (5)$$

Values are reported as percentages (the asymmetry multiplied by 100) with the statistical uncertainty as a superscript and the systematic uncertainty as a subscript:  $A_{\text{LU}}^{\text{stat}}_{\text{sys}}$ .

| Bin | $\langle x \rangle$ | $A_{LU}^{\sin(\phi_h)}$      | $A_{LU}^{\sin(\phi_h - \phi_{R\perp})}$ | $A_{LU}^{\sin(\phi_{R\perp})}$ | $A_{LU}^{\sin(2\phi_h - \phi_{R\perp})}$ | $A_{LU}^{\sin(2\phi_h - 2\phi_{R\perp})}$ | $A_{LU}^{\sin(-\phi_h + 2\phi_{R\perp})}$ | $A_{LU}^{\sin(3\phi_h - 2\phi_{R\perp})}$ |
|-----|---------------------|------------------------------|-----------------------------------------|--------------------------------|------------------------------------------|-------------------------------------------|-------------------------------------------|-------------------------------------------|
| 1   | 0.105               | $1.03_{\pm 0.11}^{\pm 0.54}$ | $-2.42_{\pm 0.11}^{\pm 0.45}$           | $1.30_{\pm 0.08}^{\pm 0.51}$   | $-0.80_{\pm 0.05}^{\pm 0.48}$            | $1.84_{\pm 0.11}^{\pm 0.47}$              | $-2.39_{\pm 0.13}^{\pm 0.43}$             | $0.69_{\pm 0.05}^{\pm 0.42}$              |
| 2   | 0.127               | $2.28_{\pm 0.15}^{\pm 0.54}$ | $-2.23_{\pm 0.12}^{\pm 0.47}$           | $2.03_{\pm 0.09}^{\pm 0.51}$   | $-0.61_{\pm 0.05}^{\pm 0.48}$            | $1.65_{\pm 0.12}^{\pm 0.48}$              | $-1.26_{\pm 0.07}^{\pm 0.44}$             | $1.25_{\pm 0.09}^{\pm 0.42}$              |
| 3   | 0.143               | $1.84_{\pm 0.14}^{\pm 0.54}$ | $-1.58_{\pm 0.09}^{\pm 0.49}$           | $2.50_{\pm 0.12}^{\pm 0.51}$   | $-1.00_{\pm 0.10}^{\pm 0.48}$            | $1.12_{\pm 0.09}^{\pm 0.49}$              | $-1.36_{\pm 0.07}^{\pm 0.45}$             | $0.62_{\pm 0.05}^{\pm 0.43}$              |
| 4   | 0.157               | $2.63_{\pm 0.17}^{\pm 0.52}$ | $-1.70_{\pm 0.10}^{\pm 0.49}$           | $2.58_{\pm 0.12}^{\pm 0.50}$   | $-0.21_{\pm 0.12}^{\pm 0.47}$            | $0.76_{\pm 0.14}^{\pm 0.49}$              | $-1.05_{\pm 0.17}^{\pm 0.45}$             | $0.83_{\pm 0.04}^{\pm 0.42}$              |
| 5   | 0.174               | $2.22_{\pm 0.14}^{\pm 0.48}$ | $-2.03_{\pm 0.10}^{\pm 0.46}$           | $2.72_{\pm 0.13}^{\pm 0.46}$   | $-1.15_{\pm 0.07}^{\pm 0.43}$            | $1.83_{\pm 0.14}^{\pm 0.46}$              | $-2.60_{\pm 0.16}^{\pm 0.41}$             | $0.88_{\pm 0.10}^{\pm 0.39}$              |
| 6   | 0.191               | $1.74_{\pm 0.15}^{\pm 0.51}$ | $-1.85_{\pm 0.11}^{\pm 0.50}$           | $2.37_{\pm 0.11}^{\pm 0.49}$   | $-1.72_{\pm 0.12}^{\pm 0.46}$            | $1.61_{\pm 0.13}^{\pm 0.49}$              | $-1.78_{\pm 0.08}^{\pm 0.44}$             | $-0.15_{\pm 0.11}^{\pm 0.41}$             |
| 7   | 0.211               | $2.58_{\pm 0.20}^{\pm 0.45}$ | $-1.23_{\pm 0.09}^{\pm 0.46}$           | $2.00_{\pm 0.10}^{\pm 0.44}$   | $-1.26_{\pm 0.08}^{\pm 0.41}$            | $1.71_{\pm 0.15}^{\pm 0.45}$              | $-1.68_{\pm 0.07}^{\pm 0.40}$             | $0.53_{\pm 0.03}^{\pm 0.38}$              |
| 8   | 0.235               | $1.51_{\pm 0.14}^{\pm 0.47}$ | $-1.09_{\pm 0.11}^{\pm 0.48}$           | $2.46_{\pm 0.14}^{\pm 0.45}$   | $-1.01_{\pm 0.07}^{\pm 0.43}$            | $1.24_{\pm 0.13}^{\pm 0.47}$              | $-1.53_{\pm 0.07}^{\pm 0.42}$             | $0.45_{\pm 0.06}^{\pm 0.39}$              |
| 9   | 0.261               | $2.09_{\pm 0.17}^{\pm 0.49}$ | $-0.56_{\pm 0.12}^{\pm 0.52}$           | $1.76_{\pm 0.11}^{\pm 0.47}$   | $-0.62_{\pm 0.09}^{\pm 0.45}$            | $1.62_{\pm 0.18}^{\pm 0.50}$              | $-1.24_{\pm 0.07}^{\pm 0.45}$             | $1.06_{\pm 0.14}^{\pm 0.41}$              |
| 10  | 0.294               | $1.52_{\pm 0.25}^{\pm 0.45}$ | $-0.77_{\pm 0.16}^{\pm 0.50}$           | $2.22_{\pm 0.15}^{\pm 0.44}$   | $-1.20_{\pm 0.08}^{\pm 0.43}$            | $0.82_{\pm 0.12}^{\pm 0.47}$              | $-1.56_{\pm 0.08}^{\pm 0.42}$             | $0.02_{\pm 0.03}^{\pm 0.39}$              |
| 11  | 0.342               | $3.61_{\pm 0.31}^{\pm 0.46}$ | $-2.05_{\pm 0.29}^{\pm 0.52}$           | $3.26_{\pm 0.24}^{\pm 0.45}$   | $-1.21_{\pm 0.10}^{\pm 0.44}$            | $1.07_{\pm 0.16}^{\pm 0.49}$              | $-1.62_{\pm 0.13}^{\pm 0.43}$             | $-0.08_{\pm 0.09}^{\pm 0.40}$             |
| 12  | 0.441               | $2.49_{\pm 0.25}^{\pm 0.46}$ | $0.10_{\pm 0.18}^{\pm 0.54}$            | $2.03_{\pm 0.15}^{\pm 0.45}$   | $-0.77_{\pm 0.08}^{\pm 0.45}$            | $0.40_{\pm 0.13}^{\pm 0.50}$              | $-0.68_{\pm 0.07}^{\pm 0.45}$             | $0.70_{\pm 0.05}^{\pm 0.41}$              |

TABLE I: The mean value of  $x$  and the final beam spin asymmetries as a function of  $x$  in each bin for each of the seven azimuthal modulations. Asymmetries are given as  $100A_{LU}^{\text{stat}}_{\text{sys}}$ .

| Bin | $\langle M_h \rangle$ | $A_{LU}^{\sin(\phi_h)}$ | $A_{LU}^{\sin(\phi_h - \phi_{R\perp})}$ | $A_{LU}^{\sin(\phi_{R\perp})}$ | $A_{LU}^{\sin(2\phi_h - \phi_{R\perp})}$ | $A_{LU}^{\sin(2\phi_h - 2\phi_{R\perp})}$ | $A_{LU}^{\sin(-\phi_h + 2\phi_{R\perp})}$ | $A_{LU}^{\sin(3\phi_h - 2\phi_{R\perp})}$ |
|-----|-----------------------|-------------------------|-----------------------------------------|--------------------------------|------------------------------------------|-------------------------------------------|-------------------------------------------|-------------------------------------------|
| 1   | 0.338                 | $3.46^{+0.45}_{-0.23}$  | $0.21^{+0.84}_{-0.12}$                  | $1.32^{+0.65}_{-0.09}$         | $0.20^{+0.61}_{-0.01}$                   | $-2.07^{+0.83}_{-0.11}$                   | $0.67^{+0.61}_{-0.07}$                    | $-1.32^{+0.61}_{-0.10}$                   |
| 2   | 0.422                 | $2.64^{+0.52}_{-0.17}$  | $2.18^{+0.78}_{-0.20}$                  | $-0.70^{+0.65}_{-0.09}$        | $0.03^{+0.57}_{-0.02}$                   | $-1.59^{+0.75}_{-0.08}$                   | $0.83^{+0.56}_{-0.08}$                    | $0.14^{+0.54}_{-0.05}$                    |
| 3   | 0.496                 | $2.07^{+0.61}_{-0.14}$  | $2.65^{+0.81}_{-0.24}$                  | $-0.08^{+0.72}_{-0.04}$        | $0.33^{+0.59}_{-0.07}$                   | $-1.39^{+0.78}_{-0.08}$                   | $0.27^{+0.60}_{-0.06}$                    | $-0.39^{+0.55}_{-0.04}$                   |
| 4   | 0.568                 | $2.36^{+0.62}_{-0.17}$  | $0.69^{+0.73}_{-0.17}$                  | $0.94^{+0.70}_{-0.06}$         | $-1.19^{+0.55}_{-0.10}$                  | $-1.96^{+0.71}_{-0.17}$                   | $-0.14^{+0.57}_{-0.07}$                   | $-0.22^{+0.50}_{-0.06}$                   |
| 5   | 0.641                 | $1.48^{+0.63}_{-0.13}$  | $2.08^{+0.67}_{-0.29}$                  | $0.64^{+0.66}_{-0.07}$         | $-0.64^{+0.52}_{-0.08}$                  | $1.22^{+0.64}_{-0.13}$                    | $-1.74^{+0.53}_{-0.10}$                   | $1.16^{+0.47}_{-0.11}$                    |
| 6   | 0.708                 | $2.07^{+0.57}_{-0.14}$  | $-1.20^{+0.56}_{-0.10}$                 | $1.79^{+0.56}_{-0.08}$         | $-1.52^{+0.47}_{-0.11}$                  | $2.25^{+0.54}_{-0.18}$                    | $-1.89^{+0.46}_{-0.11}$                   | $0.15^{+0.41}_{-0.07}$                    |
| 7   | 0.759                 | $2.25^{+0.59}_{-0.14}$  | $-2.62^{+0.57}_{-0.12}$                 | $2.57^{+0.56}_{-0.12}$         | $-0.85^{+0.49}_{-0.07}$                  | $4.36^{+0.55}_{-0.29}$                    | $-3.26^{+0.48}_{-0.20}$                   | $0.82^{+0.42}_{-0.08}$                    |
| 8   | 0.805                 | $2.07^{+0.56}_{-0.14}$  | $-2.98^{+0.52}_{-0.13}$                 | $2.58^{+0.52}_{-0.12}$         | $-0.93^{+0.47}_{-0.07}$                  | $4.21^{+0.51}_{-0.28}$                    | $-2.24^{+0.45}_{-0.11}$                   | $0.26^{+0.41}_{-0.04}$                    |
| 9   | 0.864                 | $2.36^{+0.50}_{-0.18}$  | $-3.51^{+0.46}_{-0.17}$                 | $2.45^{+0.45}_{-0.13}$         | $-0.22^{+0.42}_{-0.07}$                  | $2.00^{+0.45}_{-0.17}$                    | $-1.91^{+0.41}_{-0.09}$                   | $0.32^{+0.38}_{-0.02}$                    |
| 10  | 0.939                 | $0.70^{+0.48}_{-0.10}$  | $-3.10^{+0.43}_{-0.18}$                 | $3.14^{+0.42}_{-0.18}$         | $-0.96^{+0.42}_{-0.07}$                  | $1.25^{+0.43}_{-0.13}$                    | $-1.50^{+0.40}_{-0.08}$                   | $0.55^{+0.37}_{-0.04}$                    |
| 11  | 1.045                 | $1.01^{+0.42}_{-0.10}$  | $-1.00^{+0.37}_{-0.12}$                 | $2.68^{+0.36}_{-0.14}$         | $-0.72^{+0.38}_{-0.06}$                  | $1.19^{+0.38}_{-0.12}$                    | $-1.08^{+0.37}_{-0.05}$                   | $0.29^{+0.35}_{-0.02}$                    |
| 12  | 1.271                 | $-0.43^{+0.38}_{-0.05}$ | $-1.95^{+0.35}_{-0.10}$                 | $4.17^{+0.33}_{-0.20}$         | $0.39^{+0.36}_{-0.02}$                   | $2.41^{+0.36}_{-0.20}$                    | $-1.10^{+0.36}_{-0.05}$                   | $0.44^{+0.35}_{-0.02}$                    |

TABLE II: The mean value of  $M_h$  (given in GeV) and the final beam spin asymmetries as a function of  $M_h$  in each bin for each of the seven azimuthal modulations. Asymmetries are given as

$$100A_{LU}^{\text{stat}}_{\text{sys}}.$$

| Bin | $\langle z \rangle$ | $A_{LU}^{\sin(\phi_h)}$ | $A_{LU}^{\sin(\phi_h - \phi_{R\perp})}$ | $A_{LU}^{\sin(\phi_{R\perp})}$ | $A_{LU}^{\sin(2\phi_h - \phi_{R\perp})}$ | $A_{LU}^{\sin(2\phi_h - 2\phi_{R\perp})}$ | $A_{LU}^{\sin(-\phi_h + 2\phi_{R\perp})}$ | $A_{LU}^{\sin(3\phi_h - 2\phi_{R\perp})}$ |
|-----|---------------------|-------------------------|-----------------------------------------|--------------------------------|------------------------------------------|-------------------------------------------|-------------------------------------------|-------------------------------------------|
| 1   | 0.400               | $3.13^{+0.68}_{-0.25}$  | $-1.38^{+0.81}_{-0.18}$                 | $1.90^{+0.78}_{-0.16}$         | $-1.31^{+0.67}_{-0.13}$                  | $-1.79^{+0.83}_{-0.14}$                   | $1.13^{+0.66}_{-0.13}$                    | $-0.28^{+0.62}_{-0.05}$                   |
| 2   | 0.474               | $2.52^{+0.65}_{-0.17}$  | $0.55^{+0.89}_{-0.27}$                  | $0.85^{+0.79}_{-0.10}$         | $-0.20^{+0.67}_{-0.12}$                  | $-2.50^{+0.88}_{-0.23}$                   | $-0.05^{+0.69}_{-0.05}$                   | $-0.77^{+0.65}_{-0.12}$                   |
| 3   | 0.528               | $1.96^{+0.59}_{-0.14}$  | $3.56^{+0.86}_{-0.32}$                  | $-0.21^{+0.74}_{-0.14}$        | $1.27^{+0.63}_{-0.19}$                   | $-0.90^{+0.83}_{-0.08}$                   | $0.13^{+0.64}_{-0.06}$                    | $0.23^{+0.61}_{-0.03}$                    |
| 4   | 0.579               | $2.47^{+0.63}_{-0.25}$  | $2.39^{+0.94}_{-0.22}$                  | $0.83^{+0.79}_{-0.07}$         | $-0.00^{+0.68}_{-0.04}$                  | $-1.08^{+0.89}_{-0.19}$                   | $-0.25^{+0.69}_{-0.16}$                   | $0.25^{+0.66}_{-0.09}$                    |
| 5   | 0.638               | $3.90^{+0.58}_{-0.30}$  | $1.88^{+0.89}_{-0.24}$                  | $0.55^{+0.72}_{-0.14}$         | $0.04^{+0.64}_{-0.02}$                   | $-2.43^{+0.82}_{-0.11}$                   | $0.81^{+0.64}_{-0.12}$                    | $-0.40^{+0.61}_{-0.10}$                   |
| 6   | 0.727               | $2.65^{+0.71}_{-0.22}$  | $2.34^{+1.11}_{-0.32}$                  | $-0.71^{+0.85}_{-0.09}$        | $-0.03^{+0.75}_{-0.02}$                  | $-3.07^{+0.98}_{-0.11}$                   | $1.51^{+0.75}_{-0.17}$                    | $-1.24^{+0.69}_{-0.11}$                   |

TABLE III: The mean value of  $z$  and the final beam spin asymmetries as a function of  $z$  in each bin for  $M_h < 0.63$  GeV for each of the seven azimuthal modulations. Asymmetries are given as

$$100A_{LU}^{\text{stat}}_{\text{sys}}.$$

| Bin | $\langle z \rangle$ | $A_{LU}^{\sin(\phi_h)}$   | $A_{LU}^{\sin(\phi_h - \phi_{R\perp})}$ | $A_{LU}^{\sin(\phi_{R\perp})}$ | $A_{LU}^{\sin(2\phi_h - \phi_{R\perp})}$ | $A_{LU}^{\sin(2\phi_h - 2\phi_{R\perp})}$ | $A_{LU}^{\sin(-\phi_h + 2\phi_{R\perp})}$ | $A_{LU}^{\sin(3\phi_h - 2\phi_{R\perp})}$ |
|-----|---------------------|---------------------------|-----------------------------------------|--------------------------------|------------------------------------------|-------------------------------------------|-------------------------------------------|-------------------------------------------|
| 1   | 0.404               | $1.43_{\pm 0.12}^{+0.70}$ | $-2.33_{\pm 0.17}^{+0.43}$              | $2.27_{\pm 0.21}^{+0.64}$      | $-0.90_{\pm 0.09}^{+0.63}$               | $2.67_{\pm 0.21}^{+0.49}$                 | $-2.45_{\pm 0.18}^{+0.58}$                | $0.12_{\pm 0.08}^{+0.55}$                 |
| 2   | 0.474               | $1.90_{\pm 0.15}^{+0.67}$ | $-2.66_{\pm 0.15}^{+0.48}$              | $3.81_{\pm 0.22}^{+0.60}$      | $-1.69_{\pm 0.19}^{+0.59}$               | $2.95_{\pm 0.19}^{+0.49}$                 | $-1.87_{\pm 0.15}^{+0.55}$                | $-0.86_{\pm 0.18}^{+0.53}$                |
| 3   | 0.528               | $3.00_{\pm 0.17}^{+0.61}$ | $-2.52_{\pm 0.12}^{+0.40}$              | $4.18_{\pm 0.21}^{+0.55}$      | $-0.26_{\pm 0.10}^{+0.40}$               | $3.08_{\pm 0.19}^{+0.45}$                 | $-2.82_{\pm 0.13}^{+0.45}$                | $0.64_{\pm 0.08}^{+0.44}$                 |
| 4   | 0.580               | $2.87_{\pm 0.17}^{+0.55}$ | $-2.56_{\pm 0.11}^{+0.46}$              | $3.70_{\pm 0.22}^{+0.54}$      | $-0.93_{\pm 0.12}^{+0.58}$               | $3.31_{\pm 0.22}^{+0.49}$                 | $-2.92_{\pm 0.15}^{+0.54}$                | $0.18_{\pm 0.18}^{+0.52}$                 |
| 5   | 0.638               | $2.70_{\pm 0.22}^{+0.54}$ | $-2.46_{\pm 0.11}^{+0.45}$              | $4.79_{\pm 0.22}^{+0.51}$      | $-1.98_{\pm 0.15}^{+0.52}$               | $3.88_{\pm 0.37}^{+0.46}$                 | $-2.28_{\pm 0.12}^{+0.50}$                | $1.59_{\pm 0.10}^{+0.47}$                 |
| 6   | 0.731               | $1.40_{\pm 0.16}^{+0.57}$ | $-2.93_{\pm 0.11}^{+0.49}$              | $5.12_{\pm 0.26}^{+0.52}$      | $-1.25_{\pm 0.10}^{+0.51}$               | $1.55_{\pm 0.21}^{+0.46}$                 | $-2.92_{\pm 0.11}^{+0.51}$                | $1.21_{\pm 0.05}^{+0.47}$                 |

TABLE IV: The mean value of  $z$  and the final beam spin asymmetries as a function of  $z$  in each bin for  $M_h > 0.63$  GeV for each of the seven azimuthal modulations. Asymmetries are given as

$$100A_{LU}^{\text{stat}}_{\text{sys}}.$$

| Bin | $\langle P_h^\perp \rangle$ | $A_{LU}^{\sin(\phi_h)}$   | $A_{LU}^{\sin(\phi_h - \phi_{R\perp})}$ | $A_{LU}^{\sin(\phi_{R\perp})}$ | $A_{LU}^{\sin(2\phi_h - \phi_{R\perp})}$ | $A_{LU}^{\sin(2\phi_h - 2\phi_{R\perp})}$ | $A_{LU}^{\sin(-\phi_h + 2\phi_{R\perp})}$ | $A_{LU}^{\sin(3\phi_h - 2\phi_{R\perp})}$ |
|-----|-----------------------------|---------------------------|-----------------------------------------|--------------------------------|------------------------------------------|-------------------------------------------|-------------------------------------------|-------------------------------------------|
| 1   | 0.169                       | $0.77_{\pm 0.09}^{+1.11}$ | $0.56_{\pm 0.15}^{+1.47}$               | $1.34_{\pm 0.11}^{+0.88}$      | $1.20_{\pm 0.11}^{+0.93}$                | $-1.77_{\pm 0.18}^{+1.02}$                | $0.74_{\pm 0.10}^{+1.04}$                 | $-0.41_{\pm 0.05}^{+0.74}$                |
| 2   | 0.311                       | $0.60_{\pm 0.09}^{+1.07}$ | $2.01_{\pm 0.24}^{+1.51}$               | $-0.30_{\pm 0.13}^{+1.19}$     | $-0.70_{\pm 0.21}^{+0.89}$               | $1.53_{\pm 0.37}^{+1.20}$                 | $-0.03_{\pm 0.09}^{+0.93}$                | $0.06_{\pm 0.04}^{+0.77}$                 |
| 3   | 0.426                       | $1.84_{\pm 0.15}^{+0.89}$ | $3.70_{\pm 0.36}^{+1.34}$               | $-0.99_{\pm 0.14}^{+1.09}$     | $0.84_{\pm 0.12}^{+0.79}$                | $-0.58_{\pm 0.09}^{+1.13}$                | $0.41_{\pm 0.06}^{+0.82}$                 | $0.11_{\pm 0.02}^{+0.74}$                 |
| 4   | 0.533                       | $4.10_{\pm 0.32}^{+0.75}$ | $1.55_{\pm 0.20}^{+1.16}$               | $0.80_{\pm 0.11}^{+0.96}$      | $0.65_{\pm 0.05}^{+0.74}$                | $-2.26_{\pm 0.16}^{+1.07}$                | $0.90_{\pm 0.09}^{+0.76}$                 | $-0.05_{\pm 0.02}^{+0.73}$                |
| 5   | 0.653                       | $3.64_{\pm 0.22}^{+0.56}$ | $0.07_{\pm 0.17}^{+0.88}$               | $2.19_{\pm 0.19}^{+0.73}$      | $-0.81_{\pm 0.12}^{+0.62}$               | $-3.15_{\pm 0.18}^{+0.87}$                | $0.83_{\pm 0.07}^{+0.63}$                 | $-0.46_{\pm 0.05}^{+0.63}$                |
| 6   | 0.863                       | $2.95_{\pm 0.18}^{+0.41}$ | $1.62_{\pm 0.20}^{+0.61}$               | $0.28_{\pm 0.12}^{+0.52}$      | $-0.81_{\pm 0.05}^{+0.49}$               | $-2.27_{\pm 0.10}^{+0.64}$                | $-0.01_{\pm 0.07}^{+0.49}$                | $-0.34_{\pm 0.04}^{+0.49}$                |

TABLE V: The mean value of  $P_h^\perp$  (given in GeV) and the final beam spin asymmetries as a function of  $P_h^\perp$  in each bin for  $M_h < 0.63$  GeV for each of the seven azimuthal modulations.

$$\text{Asymmetries are given as } 100A_{LU}^{\text{stat}}_{\text{sys}}.$$

| Bin | $\langle P_h^\perp \rangle$ | $A_{LU}^{\sin(\phi_h)}$ | $A_{LU}^{\sin(\phi_h - \phi_{R\perp})}$ | $A_{LU}^{\sin(\phi_{R\perp})}$ | $A_{LU}^{\sin(2\phi_h - \phi_{R\perp})}$ | $A_{LU}^{\sin(2\phi_h - 2\phi_{R\perp})}$ | $A_{LU}^{\sin(-\phi_h + 2\phi_{R\perp})}$ | $A_{LU}^{\sin(3\phi_h - 2\phi_{R\perp})}$ |
|-----|-----------------------------|-------------------------|-----------------------------------------|--------------------------------|------------------------------------------|-------------------------------------------|-------------------------------------------|-------------------------------------------|
| 1   | 0.160                       | $0.15^{+0.52}_{-0.05}$  | $-0.25^{+0.46}_{-0.11}$                 | $4.86^{+0.39}_{-0.26}$         | $-0.07^{+0.45}_{-0.03}$                  | $1.24^{+0.39}_{-0.12}$                    | $-0.71^{+0.50}_{-0.07}$                   | $1.09^{+0.41}_{-0.06}$                    |
| 2   | 0.306                       | $0.13^{+0.58}_{-0.11}$  | $-1.46^{+0.47}_{-0.11}$                 | $4.73^{+0.48}_{-0.25}$         | $-0.86^{+0.50}_{-0.11}$                  | $1.88^{+0.43}_{-0.17}$                    | $-2.21^{+0.50}_{-0.14}$                   | $0.58^{+0.44}_{-0.04}$                    |
| 3   | 0.422                       | $2.22^{+0.56}_{-0.20}$  | $-1.76^{+0.46}_{-0.11}$                 | $4.77^{+0.56}_{-0.25}$         | $0.09^{+0.55}_{-0.20}$                   | $1.08^{+0.47}_{-0.22}$                    | $-2.26^{+0.53}_{-0.10}$                   | $0.68^{+0.47}_{-0.04}$                    |
| 4   | 0.530                       | $2.49^{+0.80}_{-0.16}$  | $-2.80^{+0.55}_{-0.15}$                 | $3.30^{+0.76}_{-0.18}$         | $-2.59^{+0.67}_{-0.33}$                  | $3.66^{+0.60}_{-0.28}$                    | $-2.69^{+0.63}_{-0.11}$                   | $0.37^{+0.57}_{-0.08}$                    |
| 5   | 0.648                       | $4.01^{+0.94}_{-0.28}$  | $-2.76^{+0.59}_{-0.12}$                 | $2.75^{+0.80}_{-0.13}$         | $-0.92^{+0.56}_{-0.19}$                  | $4.92^{+0.62}_{-0.29}$                    | $-3.04^{+0.56}_{-0.13}$                   | $1.66^{+0.63}_{-0.13}$                    |
| 6   | 0.852                       | $2.77^{+1.12}_{-0.19}$  | $-2.91^{+0.63}_{-0.11}$                 | $-0.05^{+1.04}_{-0.17}$        | $-2.84^{+0.87}_{-0.19}$                  | $8.13^{+0.74}_{-0.50}$                    | $-3.58^{+0.85}_{-0.15}$                   | $1.48^{+0.75}_{-0.06}$                    |

TABLE VI: The mean value of  $P_h^\perp$  and the final beam spin asymmetries as a function of  $P_h^\perp$  in each bin for  $M_h > 0.63$  GeV for each of the seven azimuthal modulations. Asymmetries are given

$$\text{as } 100A_{LU\text{sys}}^{\text{stat}}.$$

## II. BIN DEFINITIONS AND MEAN KINEMATIC VALUES

The bin edges for the  $x$ ,  $M_h$ ,  $z$  and  $P_h^\perp$  asymmetries are reported in Tables VII-VIII. In Tables IX-XIV the mean values of  $x$ ,  $Q^2$ ,  $M_h$ ,  $z$ ,  $P_h^\perp$ ,  $\theta$ ,  $K_2$  and  $K_3$  are reported for each bin. Figs. 1-4 show plots of seven asymmetry amplitudes for each binning scheme.

| Bin | $x$            | $M_h$ (GeV)    |
|-----|----------------|----------------|
| 1   | (0.000, 0.118] | (0.270, 0.381] |
| 2   | (0.118, 0.135] | (0.381, 0.462] |
| 3   | (0.135, 0.150] | (0.462, 0.531] |
| 4   | (0.150, 0.165] | (0.531, 0.606] |
| 5   | (0.165, 0.183] | (0.606, 0.675] |
| 6   | (0.183, 0.200] | (0.675, 0.737] |
| 7   | (0.200, 0.223] | (0.737, 0.781] |
| 8   | (0.223, 0.248] | (0.781, 0.831] |
| 9   | (0.248, 0.275] | (0.831, 0.900] |
| 10  | (0.275, 0.315] | (0.900, 0.981] |
| 11  | (0.315, 0.375] | (0.981, 1.125] |
| 12  | (0.375, 1.000] | (1.125, 2.500] |

TABLE VII: Bins of the 1-D projections of the  $A_{LU}$  measurements for the variables  $x$  and  $M_h$ .

| Bin | $z$            | $P_h^\perp$ (GeV) |
|-----|----------------|-------------------|
| 1   | (0.000, 0.445] | (0.000, 0.245]    |
| 2   | (0.445, 0.500] | (0.245, 0.365]    |
| 3   | (0.500, 0.555] | (0.365, 0.480]    |
| 4   | (0.555, 0.605] | (0.480, 0.585]    |
| 5   | (0.605, 0.675] | (0.585, 0.725]    |
| 5   | (0.675, 1.000] | (0.725, 1.500]    |

TABLE VIII: Bins of the 2-D projections of the  $A_{LU}$  measurements for the variables  $z$  and  $P_h^\perp$ .

The asymmetries are determined for  $M_h < 0.63$  GeV and  $M_h > 0.63$  GeV.

| Bin | $\langle x \rangle$ | $\langle Q^2 \rangle$ (GeV <sup>2</sup> ) | $\langle M_h \rangle$ (GeV) | $\langle z \rangle$ | $\langle P_h^\perp \rangle$ (GeV) | $\langle \theta \rangle$ | $\langle K_2 \rangle$ | $\langle K_3 \rangle$ |
|-----|---------------------|-------------------------------------------|-----------------------------|---------------------|-----------------------------------|--------------------------|-----------------------|-----------------------|
| 1   | 0.105               | 1.542                                     | 0.830                       | 0.531               | 0.550                             | 1.563                    | 0.874                 | 0.699                 |
| 2   | 0.127               | 1.783                                     | 0.809                       | 0.547               | 0.530                             | 1.569                    | 0.842                 | 0.692                 |
| 3   | 0.143               | 1.953                                     | 0.794                       | 0.557               | 0.526                             | 1.567                    | 0.822                 | 0.685                 |
| 4   | 0.157               | 2.105                                     | 0.780                       | 0.559               | 0.520                             | 1.575                    | 0.805                 | 0.679                 |
| 5   | 0.174               | 2.286                                     | 0.763                       | 0.566               | 0.506                             | 1.575                    | 0.793                 | 0.673                 |
| 6   | 0.191               | 2.471                                     | 0.749                       | 0.571               | 0.500                             | 1.574                    | 0.780                 | 0.668                 |
| 7   | 0.211               | 2.707                                     | 0.743                       | 0.571               | 0.492                             | 1.575                    | 0.776                 | 0.665                 |
| 8   | 0.235               | 3.003                                     | 0.733                       | 0.572               | 0.485                             | 1.576                    | 0.776                 | 0.664                 |
| 9   | 0.261               | 3.307                                     | 0.716                       | 0.571               | 0.468                             | 1.578                    | 0.771                 | 0.662                 |
| 10  | 0.294               | 3.721                                     | 0.701                       | 0.569               | 0.460                             | 1.578                    | 0.773                 | 0.663                 |
| 11  | 0.342               | 4.337                                     | 0.679                       | 0.565               | 0.444                             | 1.585                    | 0.778                 | 0.665                 |
| 12  | 0.441               | 5.658                                     | 0.630                       | 0.547               | 0.408                             | 1.588                    | 0.796                 | 0.674                 |

TABLE IX: Average kinematic values for the 1-D  $x$  bins.  $K_2$  ( $K_3$ ) denotes the twist-2 (twist-3)  $y$ -dependent kinematic depolarization factor entering the two-pion production cross section.

| Bin | $\langle x \rangle$ | $\langle Q^2 \rangle$ (GeV <sup>2</sup> ) | $\langle M_h \rangle$ (GeV) | $\langle z \rangle$ | $\langle P_h^\perp \rangle$ (GeV) | $\langle \theta \rangle$ | $\langle K_2 \rangle$ | $\langle K_3 \rangle$ |
|-----|---------------------|-------------------------------------------|-----------------------------|---------------------|-----------------------------------|--------------------------|-----------------------|-----------------------|
| 1   | 0.249               | 3.145                                     | 0.338                       | 0.530               | 0.638                             | 1.640                    | 0.778                 | 0.664                 |
| 2   | 0.242               | 3.090                                     | 0.422                       | 0.546               | 0.589                             | 1.600                    | 0.785                 | 0.668                 |
| 3   | 0.240               | 3.057                                     | 0.496                       | 0.551               | 0.571                             | 1.576                    | 0.785                 | 0.668                 |
| 4   | 0.238               | 3.056                                     | 0.568                       | 0.555               | 0.549                             | 1.571                    | 0.789                 | 0.671                 |
| 5   | 0.233               | 3.000                                     | 0.641                       | 0.547               | 0.519                             | 1.572                    | 0.793                 | 0.671                 |
| 6   | 0.225               | 2.918                                     | 0.708                       | 0.550               | 0.494                             | 1.575                    | 0.796                 | 0.673                 |
| 7   | 0.222               | 2.893                                     | 0.759                       | 0.555               | 0.472                             | 1.575                    | 0.796                 | 0.673                 |
| 8   | 0.219               | 2.855                                     | 0.805                       | 0.559               | 0.458                             | 1.572                    | 0.798                 | 0.673                 |
| 9   | 0.216               | 2.826                                     | 0.864                       | 0.560               | 0.434                             | 1.567                    | 0.801                 | 0.676                 |
| 10  | 0.209               | 2.764                                     | 0.939                       | 0.569               | 0.417                             | 1.560                    | 0.805                 | 0.677                 |
| 11  | 0.199               | 2.665                                     | 1.045                       | 0.579               | 0.394                             | 1.559                    | 0.816                 | 0.680                 |
| 12  | 0.180               | 2.471                                     | 1.271                       | 0.628               | 0.378                             | 1.547                    | 0.832                 | 0.687                 |

TABLE X: Average kinematic values for the 1-D  $M_h$  bins.  $K_2$  ( $K_3$ ) denotes the twist-2 (twist-3)  $y$ -dependent kinematic depolarization factor entering the two-pion production cross section.

| Bin | $\langle x \rangle$ | $\langle Q^2 \rangle$ (GeV <sup>2</sup> ) | $\langle M_h \rangle$ (GeV) | $\langle z \rangle$ | $\langle P_h^\perp \rangle$ (GeV) | $\langle \theta \rangle$ | $\langle K_2 \rangle$ | $\langle K_3 \rangle$ |
|-----|---------------------|-------------------------------------------|-----------------------------|---------------------|-----------------------------------|--------------------------|-----------------------|-----------------------|
| 1   | 0.220               | 3.129                                     | 0.464                       | 0.400               | 0.598                             | 1.578                    | 0.861                 | 0.696                 |
| 2   | 0.244               | 3.210                                     | 0.468                       | 0.474               | 0.610                             | 1.583                    | 0.809                 | 0.683                 |
| 3   | 0.248               | 3.131                                     | 0.472                       | 0.528               | 0.608                             | 1.581                    | 0.780                 | 0.669                 |
| 4   | 0.254               | 3.107                                     | 0.470                       | 0.579               | 0.590                             | 1.593                    | 0.756                 | 0.655                 |
| 5   | 0.253               | 3.021                                     | 0.478                       | 0.638               | 0.556                             | 1.609                    | 0.739                 | 0.647                 |
| 6   | 0.234               | 2.825                                     | 0.482                       | 0.727               | 0.500                             | 1.627                    | 0.7941                | 0.650                 |

TABLE XI: Average kinematic values for the 2-D  $z$  bins corresponding to  $M_h < 0.63$  GeV.  $K_2$  ( $K_3$ ) denotes the twist-2 (twist-3)  $y$ -dependent kinematic depolarization factor entering the two-pion production cross section.

| Bin | $\langle x \rangle$ | $\langle Q^2 \rangle$ (GeV <sup>2</sup> ) | $\langle M_h \rangle$ (GeV) | $\langle z \rangle$ | $\langle P_h^\perp \rangle$ (GeV) | $\langle \theta \rangle$ | $\langle K_2 \rangle$ | $\langle K_3 \rangle$ |
|-----|---------------------|-------------------------------------------|-----------------------------|---------------------|-----------------------------------|--------------------------|-----------------------|-----------------------|
| 1   | 0.192               | 2.764                                     | 0.821                       | 0.404               | 0.386                             | 1.575                    | 0.867                 | 0.698                 |
| 2   | 0.209               | 2.847                                     | 0.859                       | 0.474               | 0.427                             | 1.574                    | 0.830                 | 0.688                 |
| 3   | 0.218               | 2.862                                     | 0.880                       | 0.528               | 0.451                             | 1.573                    | 0.805                 | 0.677                 |
| 4   | 0.223               | 2.850                                     | 0.900                       | 0.580               | 0.466                             | 1.566                    | 0.786                 | 0.669                 |
| 5   | 0.221               | 2.785                                     | 0.921                       | 0.638               | 0.467                             | 1.559                    | 0.773                 | 0.662                 |
| 6   | 0.202               | 2.628                                     | 0.958                       | 0.731               | 0.438                             | 1.551                    | 0.794                 | 0.671                 |

TABLE XII: Average kinematic values for the 2-D  $z$  bins corresponding to  $M_h > 0.63$  GeV.  $K_2$  ( $K_3$ ) denotes the twist-2 (twist-3)  $y$ -dependent kinematic depolarization factor entering the two-pion production cross section.

| Bin | $\langle x \rangle$ | $\langle Q^2 \rangle$ (GeV <sup>2</sup> ) | $\langle M_h \rangle$ (GeV) | $\langle z \rangle$ | $\langle P_h^\perp \rangle$ (GeV) | $\langle \theta \rangle$ | $\langle K_2 \rangle$ | $\langle K_3 \rangle$ |
|-----|---------------------|-------------------------------------------|-----------------------------|---------------------|-----------------------------------|--------------------------|-----------------------|-----------------------|
| 1   | 0.309               | 3.534                                     | 0.501                       | 0.591               | 0.169                             | 1.587                    | 0.701                 | 0.634                 |
| 2   | 0.284               | 3.429                                     | 0.493                       | 0.568               | 0.311                             | 1.588                    | 0.745                 | 0.651                 |
| 3   | 0.259               | 3.221                                     | 0.481                       | 0.553               | 0.426                             | 1.594                    | 0.766                 | 0.660                 |
| 4   | 0.244               | 3.123                                     | 0.474                       | 0.541               | 0.533                             | 1.590                    | 0.785                 | 0.668                 |
| 5   | 0.231               | 3.027                                     | 0.464                       | 0.532               | 0.653                             | 1.594                    | 0.799                 | 0.675                 |
| 6   | 0.204               | 2.759                                     | 0.454                       | 0.531               | 0.863                             | 1.598                    | 0.823                 | 0.685                 |

TABLE XIII: Average kinematic values for the 2-D  $P_h^\perp$  bins corresponding to  $M_h < 0.63$  GeV.  $K_2$  ( $K_3$ ) denotes the twist-2 (twist-3)  $y$ -dependent kinematic depolarization factor entering the two-pion production cross section.

| Bin | $\langle x \rangle$ | $\langle Q^2 \rangle$ (GeV <sup>2</sup> ) | $\langle M_h \rangle$ (GeV) | $\langle z \rangle$ | $\langle P_h^\perp \rangle$ (GeV) | $\langle \theta \rangle$ | $\langle K_2 \rangle$ | $\langle K_3 \rangle$ |
|-----|---------------------|-------------------------------------------|-----------------------------|---------------------|-----------------------------------|--------------------------|-----------------------|-----------------------|
| 1   | 0.226               | 2.897                                     | 0.946                       | 0.560               | 0.160                             | 1.556                    | 0.789                 | 0.670                 |
| 2   | 0.221               | 2.865                                     | 0.915                       | 0.566               | 0.306                             | 1.556                    | 0.796                 | 0.673                 |
| 3   | 0.217               | 2.837                                     | 0.894                       | 0.570               | 0.422                             | 1.563                    | 0.801                 | 0.676                 |
| 4   | 0.207               | 2.752                                     | 0.876                       | 0.570               | 0.530                             | 1.570                    | 0.811                 | 0.679                 |
| 5   | 0.199               | 2.677                                     | 0.858                       | 0.574               | 0.648                             | 1.572                    | 0.819                 | 0.684                 |
| 6   | 0.182               | 2.528                                     | 0.832                       | 0.586               | 0.852                             | 1.589                    | 0.839                 | 0.689                 |

TABLE XIV: Average kinematic values for the 2-D  $P_h^\perp$  bins corresponding to  $M_h > 0.63$  GeV.  $K_2$  ( $K_3$ ) denotes the twist-2 (twist-3)  $y$ -dependent kinematic depolarization factor entering the two-pion production cross section.

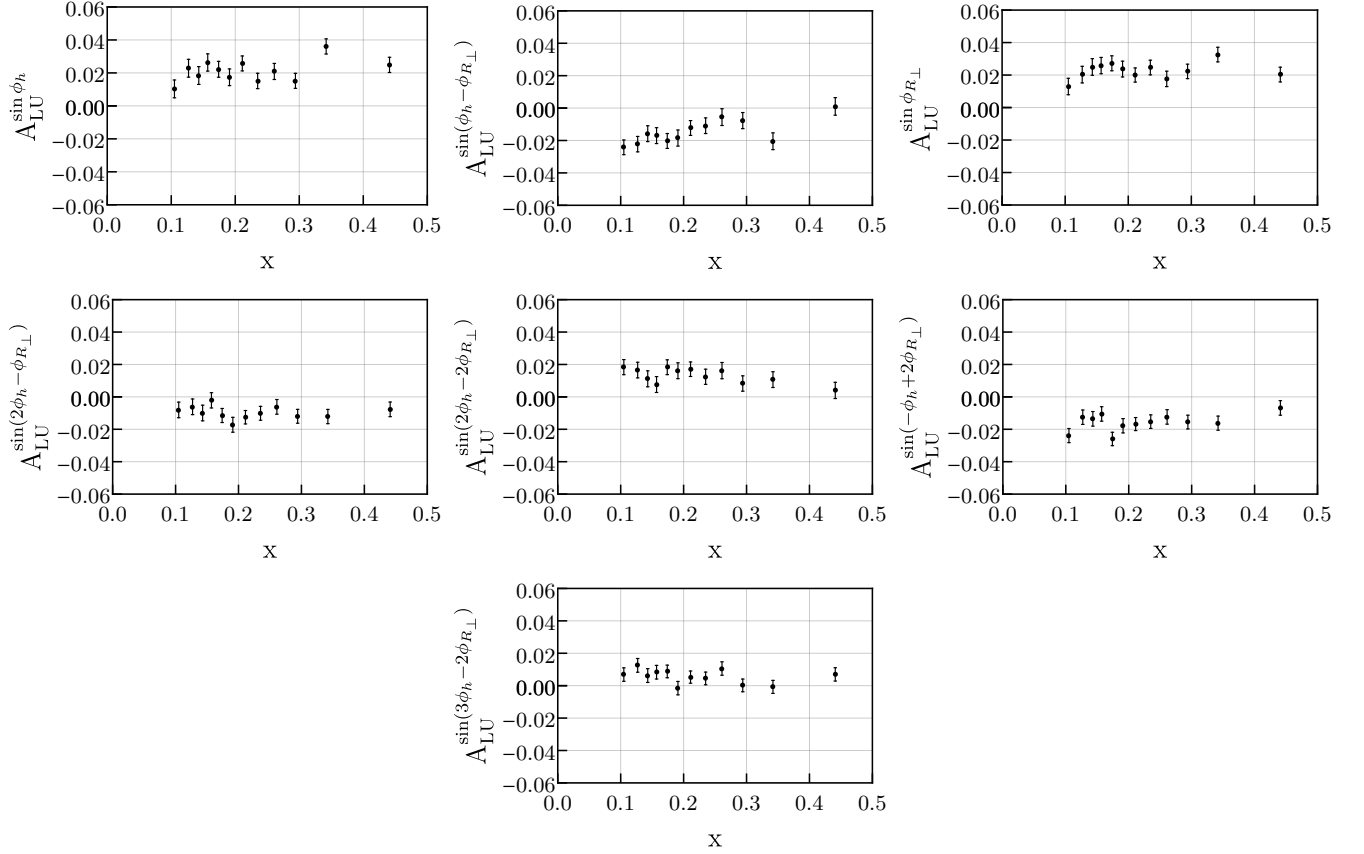

FIG. 1: The seven extracted beam spin asymmetries from the simultaneous fit to all modulations as a function of  $x$ . Error bars are purely statistical.

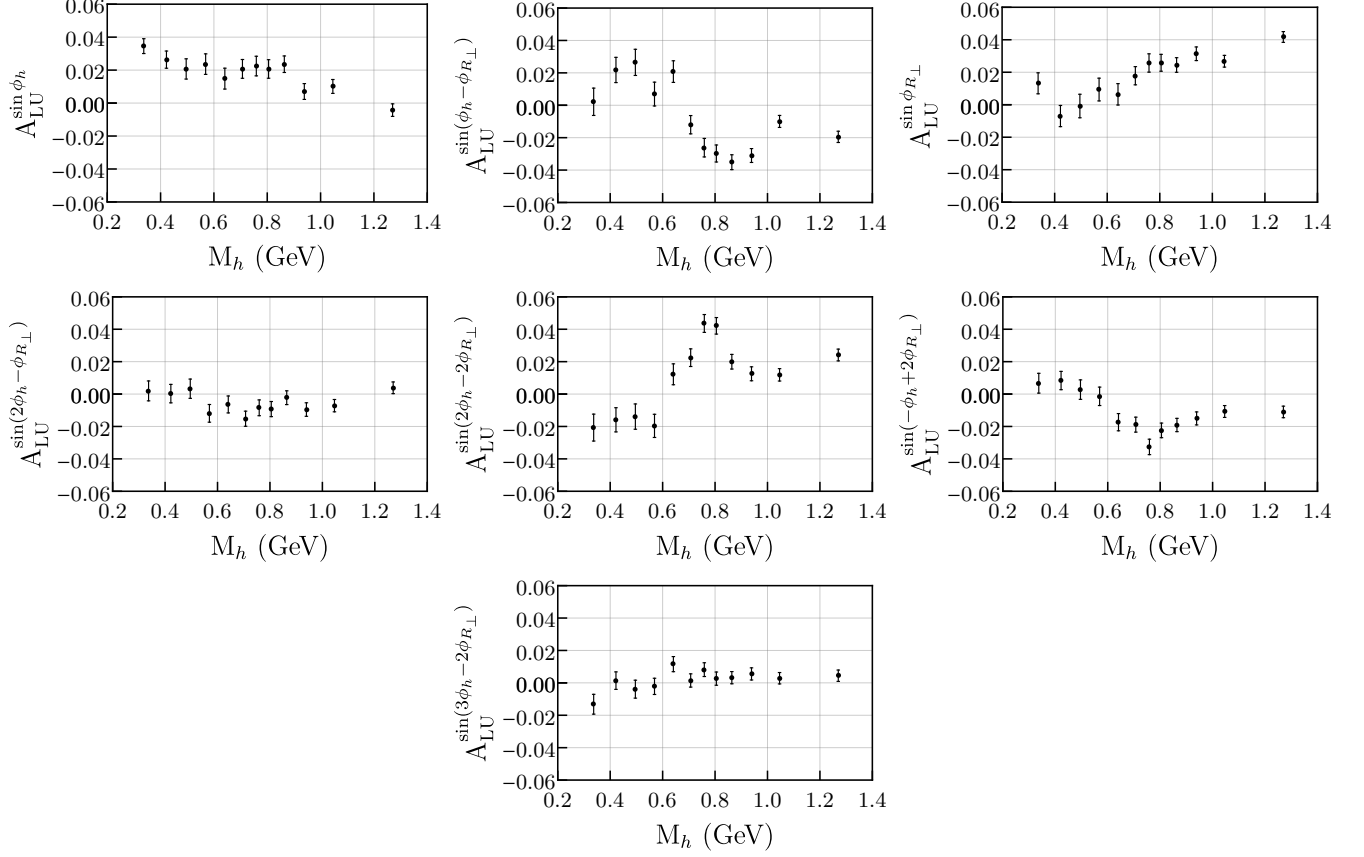

FIG. 2: The seven extracted beam spin asymmetries from the simultaneous fit to all modulations as a function of  $M_h$ . Error bars are purely statistical.

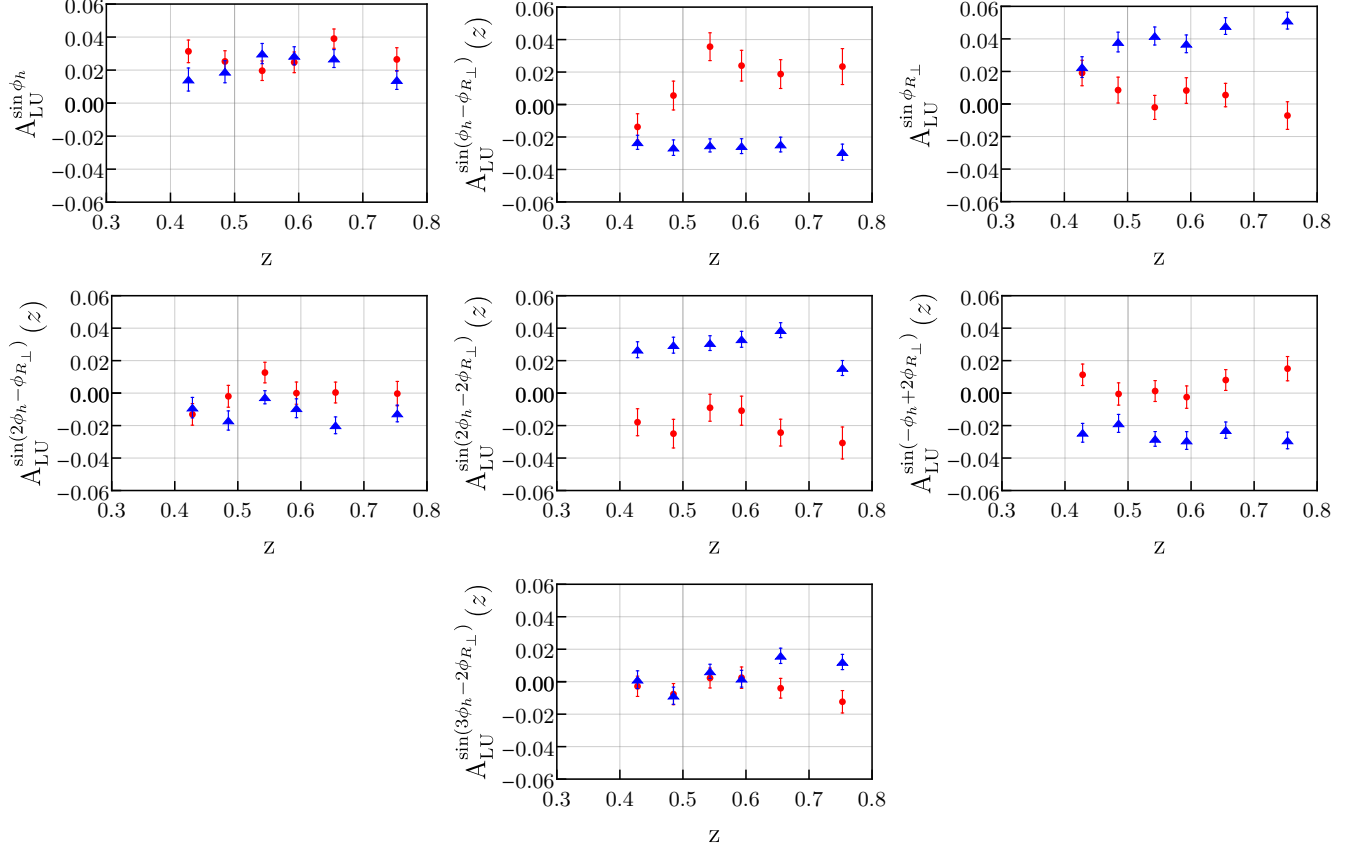

FIG. 3: The seven extracted beam spin asymmetries from the simultaneous fit to all modulations as a function of  $z$  for  $M_h < 0.63$  GeV (red circles) and  $M_h > 0.63$  GeV (blue triangles). Error bars are purely statistical.

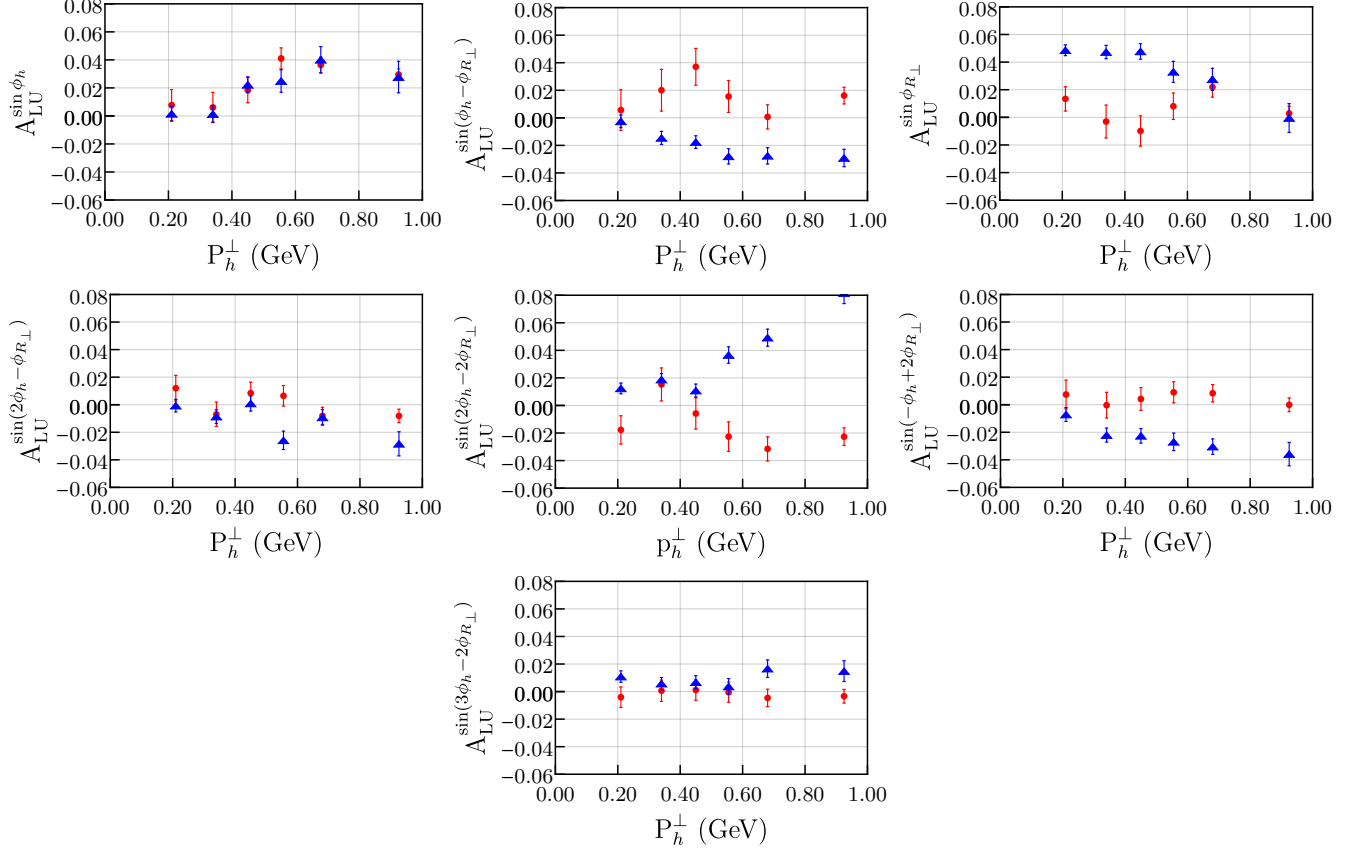

FIG. 4: The seven extracted beam spin asymmetries from the simultaneous fit to all modulations as a function of  $P_h^\perp$  (given in GeV) for  $M_h < 0.63$  GeV (red circles) and  $M_h > 0.63$  GeV (blue triangles). Error bars are purely statistical.

### III. INFLUENCE ON $A_{LU}$ FROM UNPOLARIZED CROSS SECTION MODULATIONS

The unpolarized cross section  $d\sigma_{UU}$ , which resides in the denominator of  $A_{LU}$ , also contains several modulations [3]. Limitations in the CLAS12 acceptance introduce linear dependence between the amplitudes, hence  $A_{LU}$  could be influenced by nonzero amplitudes of  $d\sigma_{UU}$  modulations. These amplitudes have not yet been measured for the relevant kinematical ranges, therefore it is difficult to correct for their impact. Instead, we assume they are no more than 10% and performed a Monte Carlo study to assess their influence on the final  $A_{LU}$  values. Figs. 5-10 show distributions of  $\delta$ , the resulting shift on an  $A_{LU}$  amplitude from nonzero  $d\sigma_{UU}$  amplitudes, for each  $A_{LU}$  measurement bin. In general,  $\delta \lesssim 0.3\%$ .

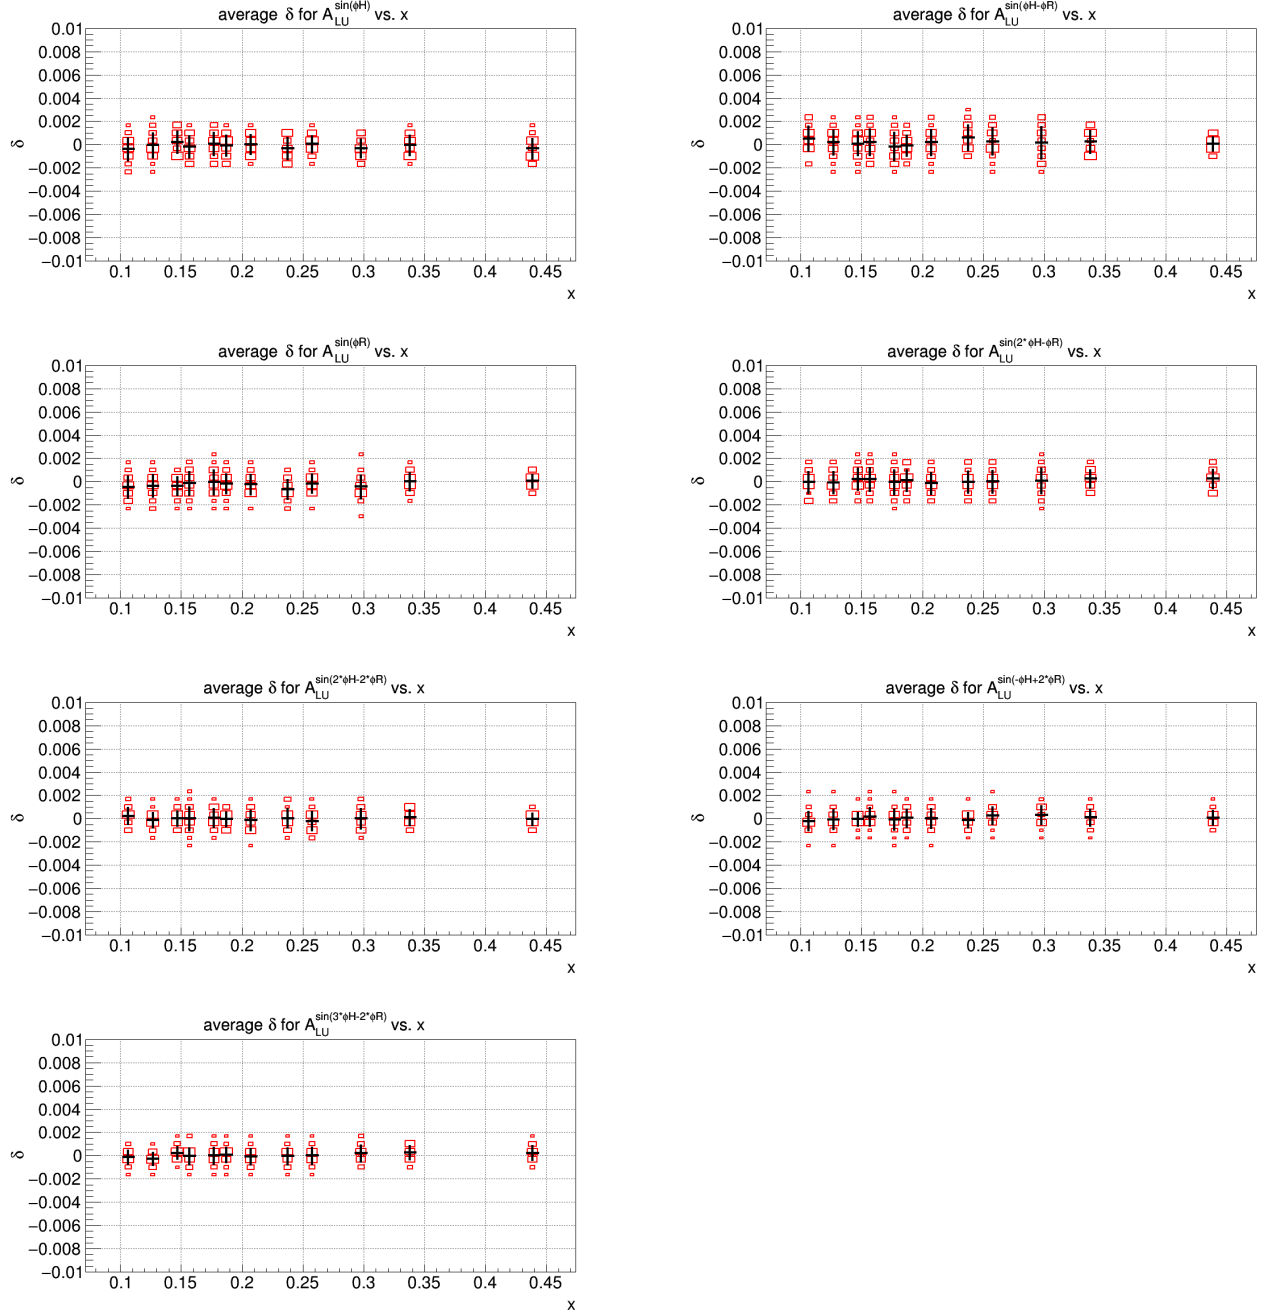

FIG. 5: Distribution of  $\delta$  for each kinematic bin and  $\sigma_{LU}$  modulation; this is for the binning in  $x$ . One histogram entry (red box plot) corresponds to one  $\sigma_{UU}$  amplitude injection; the size of the red box is proportional to the number of entries in that bin. The black crosses indicate the mean  $\delta$  for each kinematic bin, and the vertical size of the black cross indicates the standard deviation of  $\delta$ .

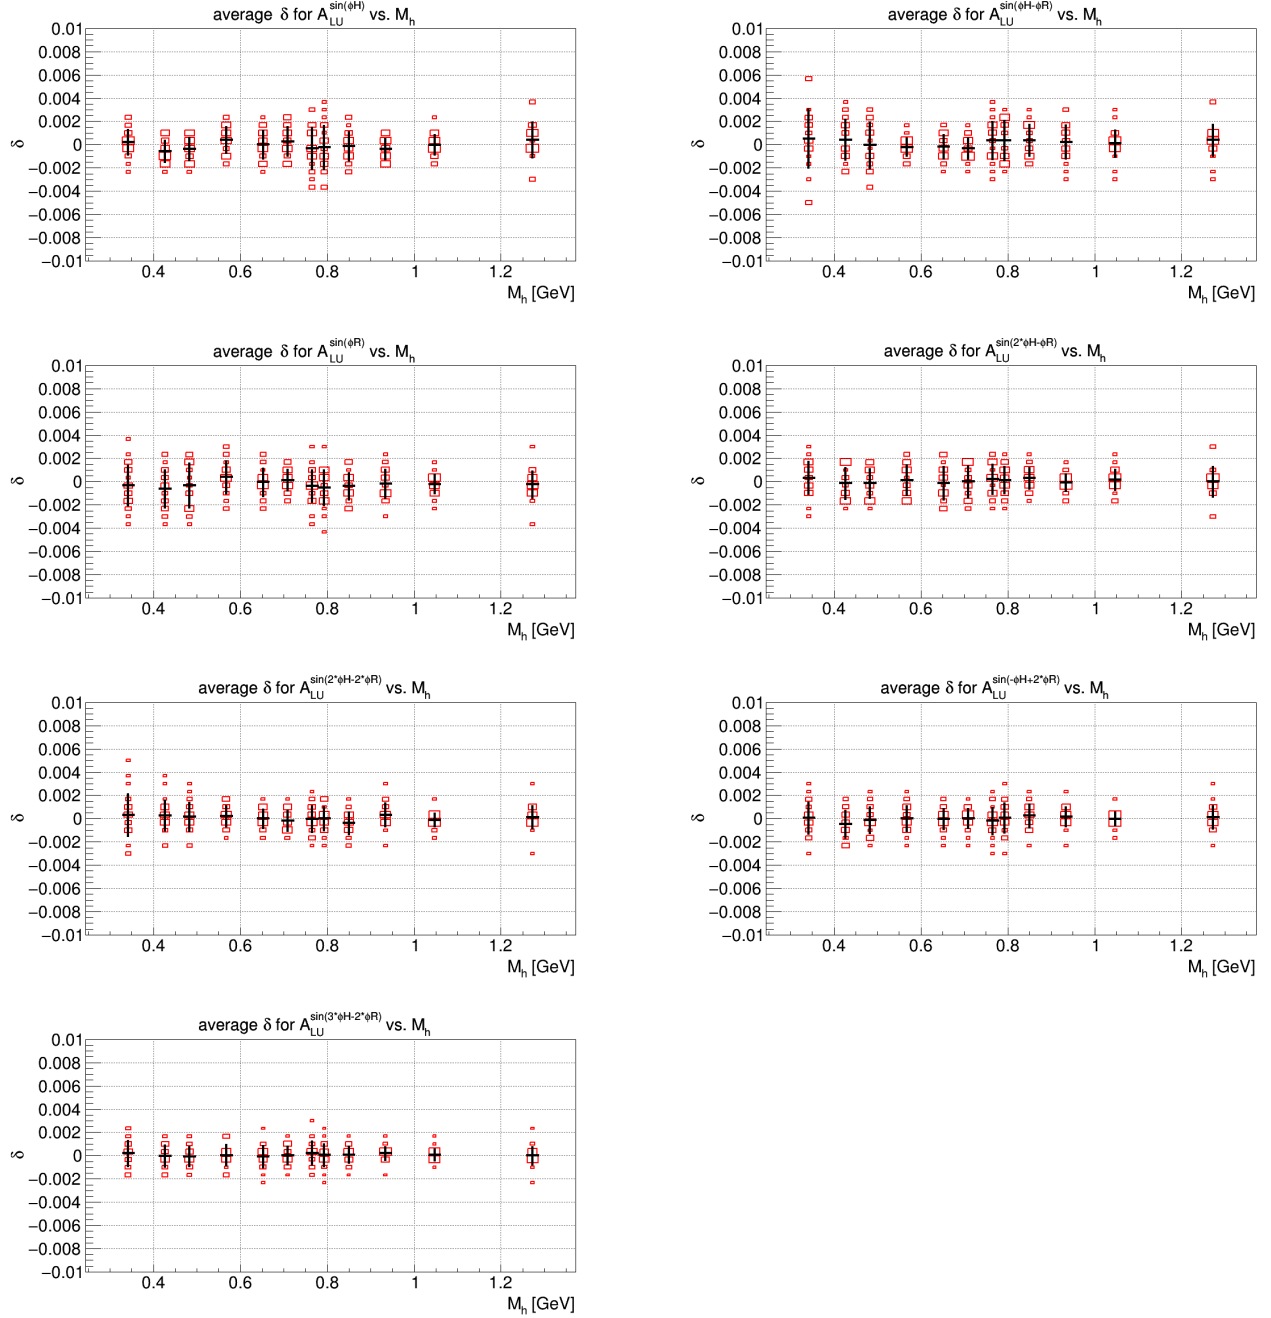

FIG. 6: Distribution of  $\delta$  for each kinematic bin and  $\sigma_{LU}$  modulation; this is for the binning in  $M_h$ . One histogram entry (red box plot) corresponds to one  $\sigma_{UU}$  amplitude injection; the size of the red box is proportional to the number of entries in that bin. The black crosses indicate the mean  $\delta$  for each kinematic bin, and the vertical size of the black cross indicates the standard deviation of  $\delta$ .

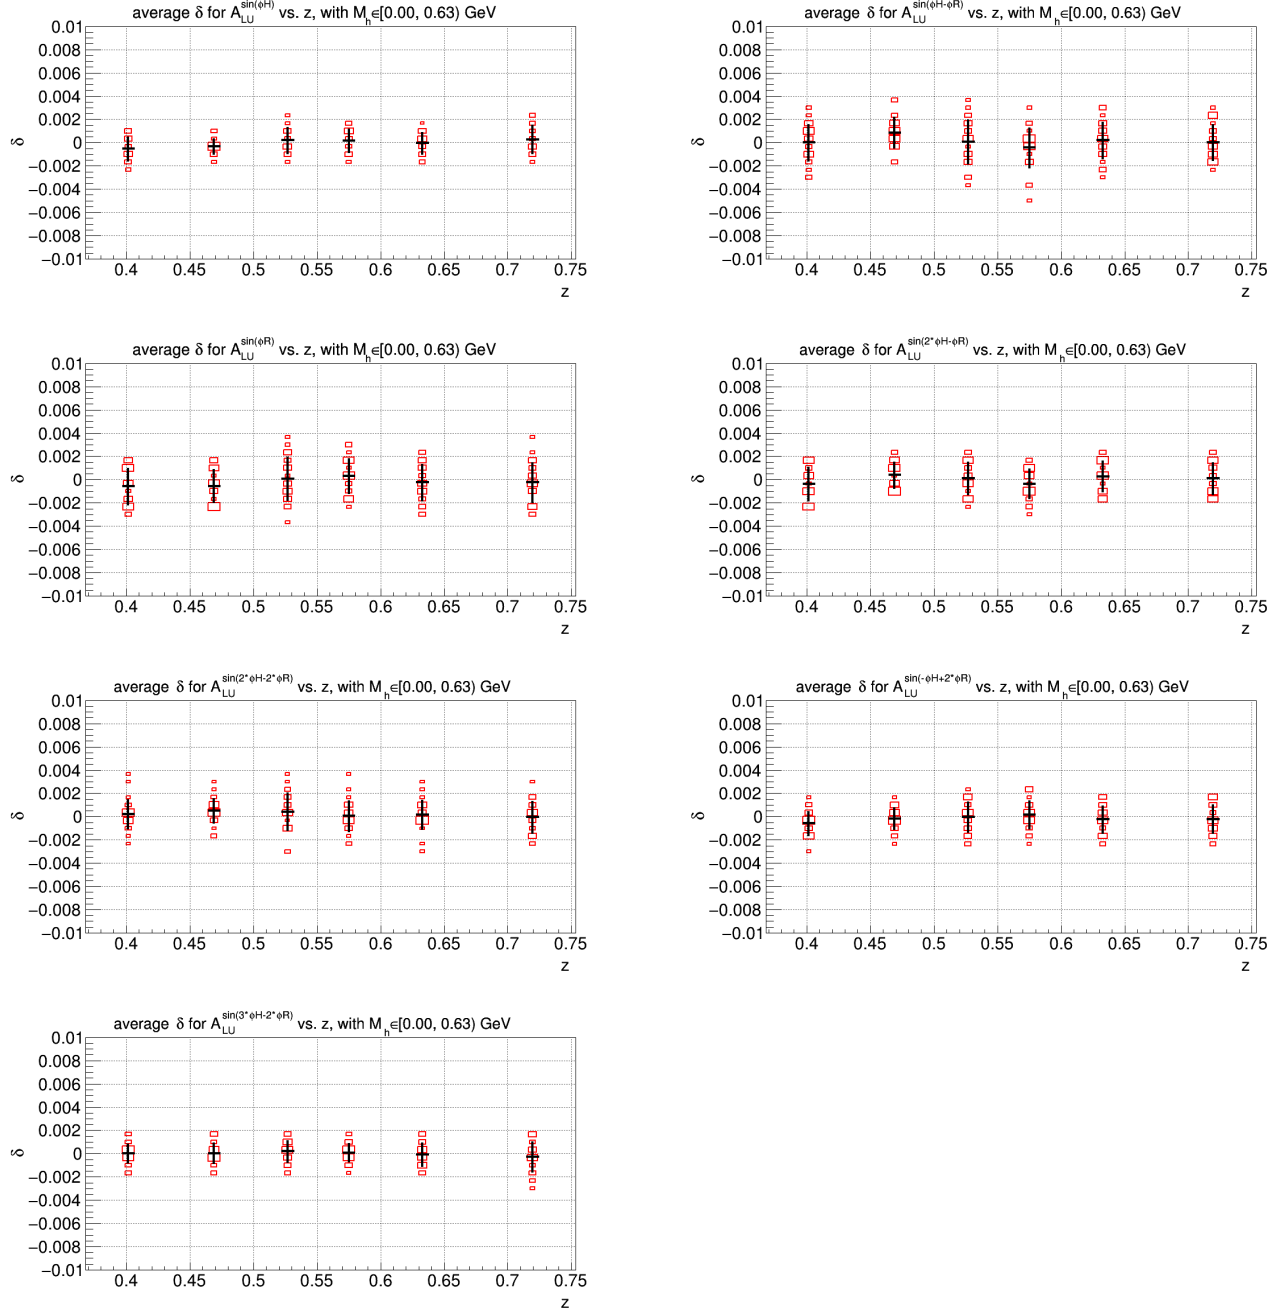

FIG. 7: Distribution of  $\delta$  for each kinematic bin and  $\sigma_{LU}$  modulation; this is for the binning in  $z$ , with  $M_h < 0.63$  GeV. One histogram entry (red box plot) corresponds to one  $\sigma_{UU}$  amplitude injection; the size of the red box is proportional to the number of entries in that bin. The black crosses indicate the mean  $\delta$  for each kinematic bin, and the vertical size of the black cross indicates the standard deviation of  $\delta$ .

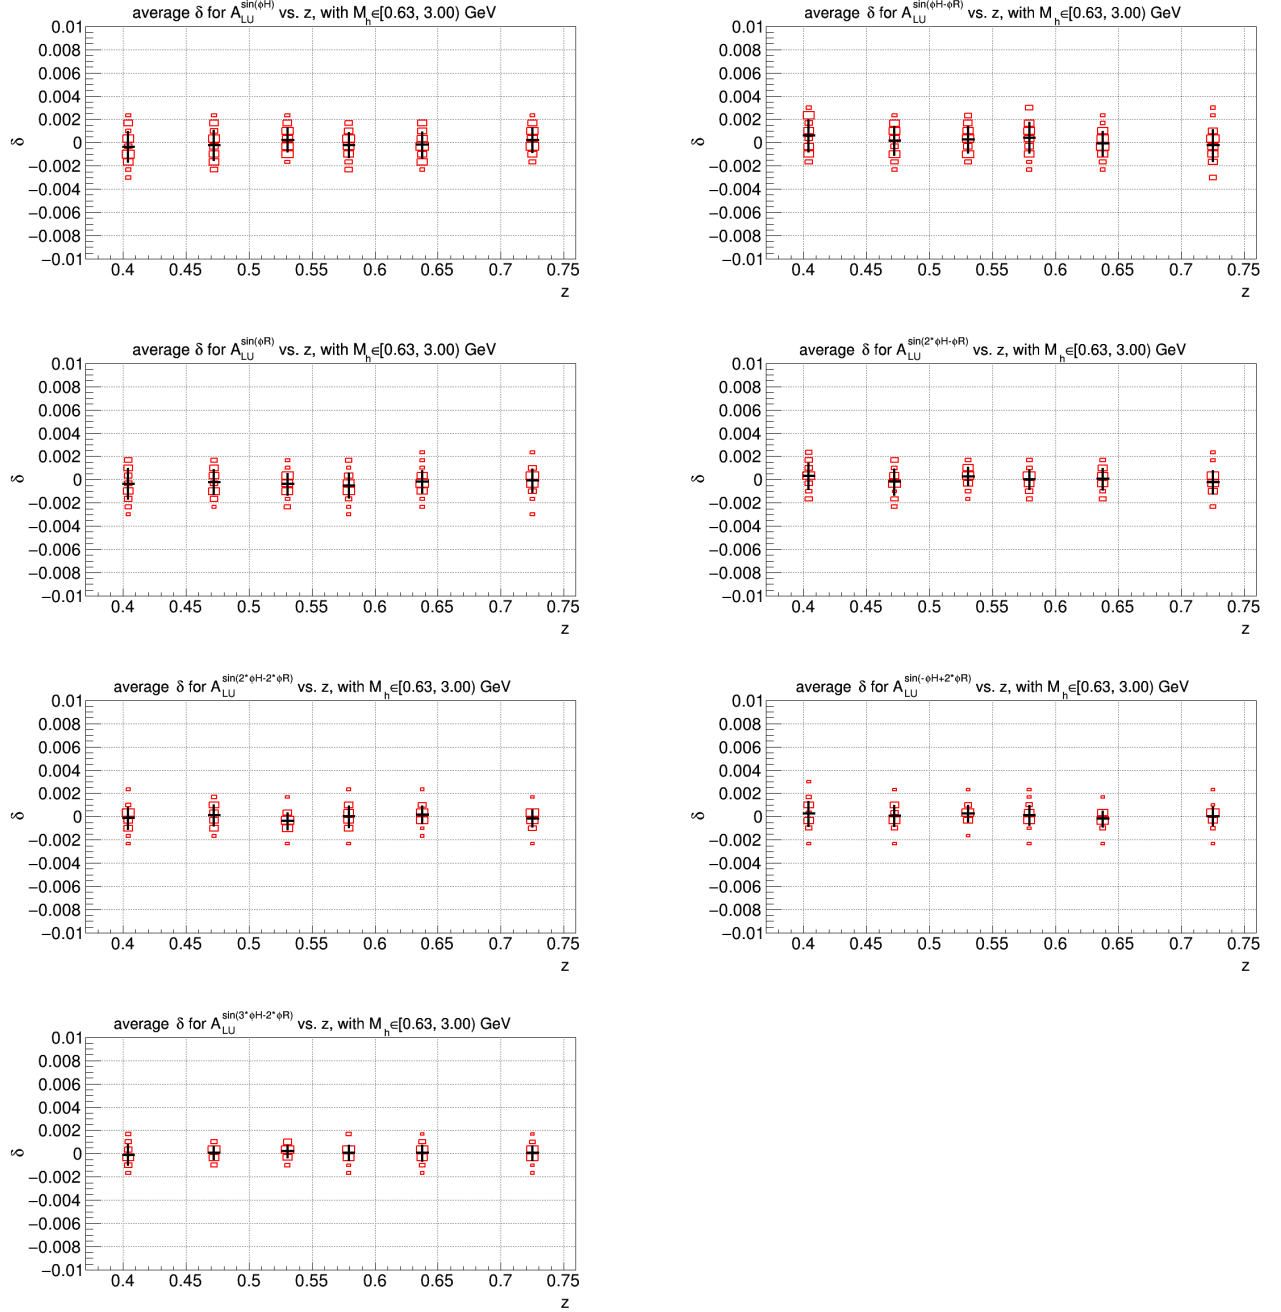

FIG. 8: Distribution of  $\delta$  for each kinematic bin and  $\sigma_{LU}$  modulation; this is for the binning in  $z$ , with  $M_h > 0.63$  GeV. One histogram entry (red box plot) corresponds to one  $\sigma_{UU}$  amplitude injection; the size of the red box is proportional to the number of entries in that bin. The black crosses indicate the mean  $\delta$  for each kinematic bin, and the vertical size of the black cross indicates the standard deviation of  $\delta$ .

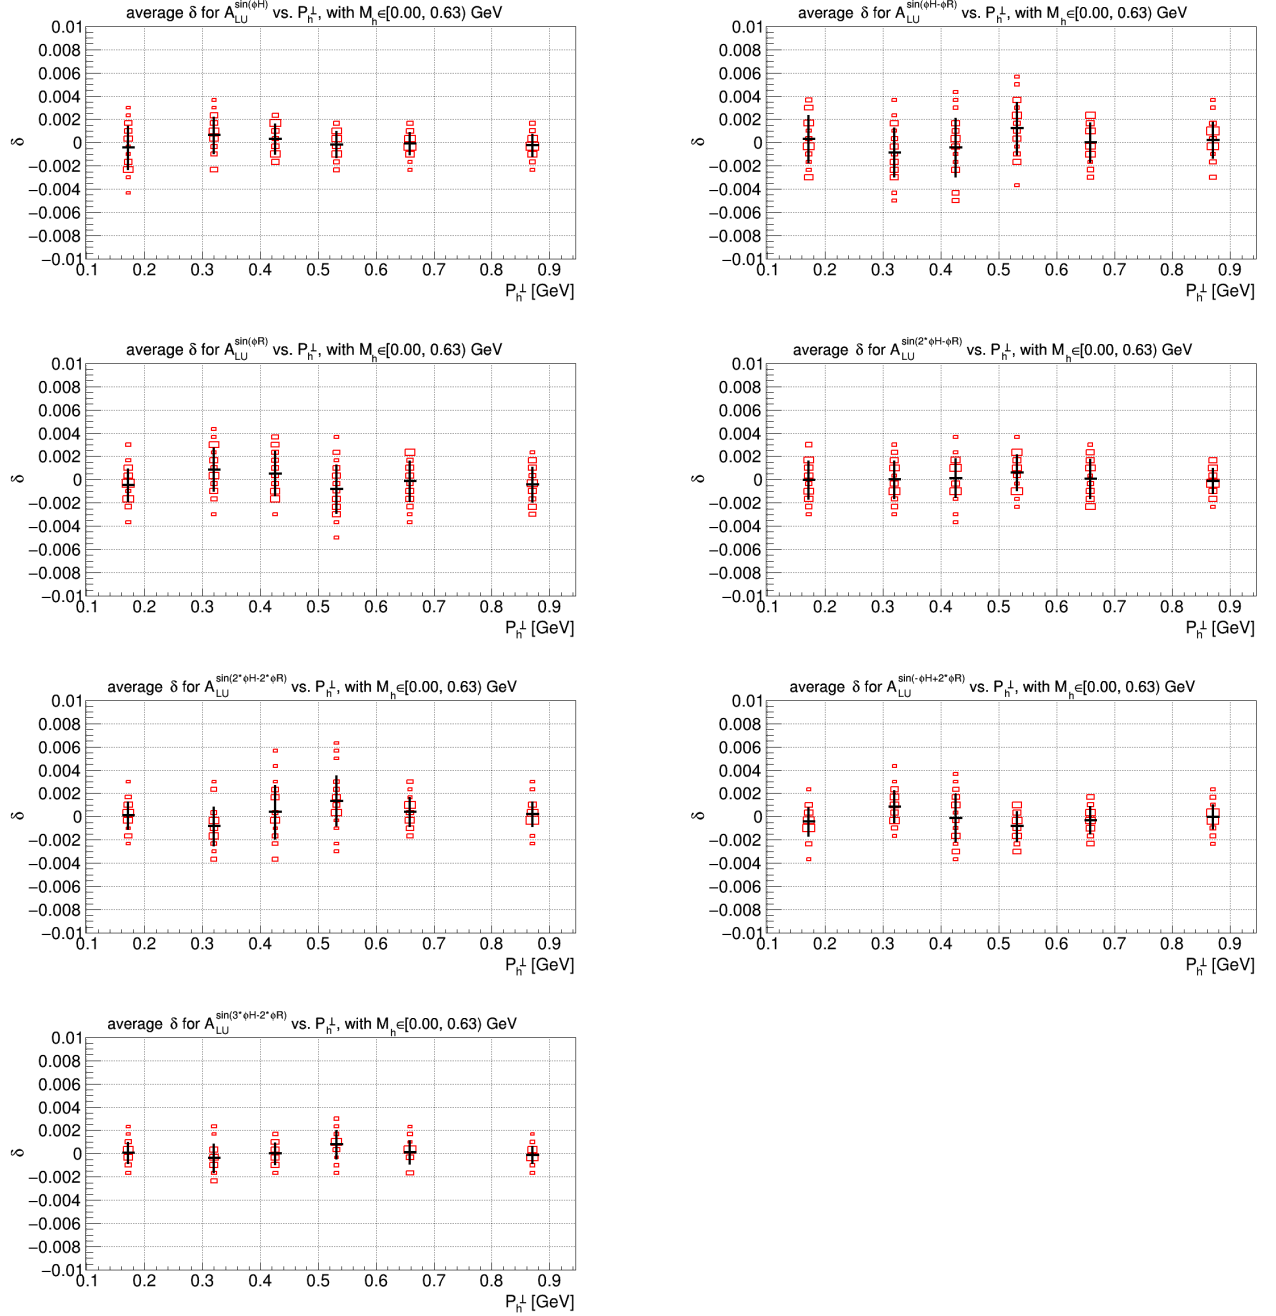

FIG. 9: Distribution of  $\delta$  for each kinematic bin and  $\sigma_{LU}$  modulation; this is for the binning in  $P_h^\perp$ , with  $M_h < 0.63$  GeV. One histogram entry (red box plot) corresponds to one  $\sigma_{UU}$  amplitude injection; the size of the red box is proportional to the number of entries in that bin. The black crosses indicate the mean  $\delta$  for each kinematic bin, and the vertical size of the black cross indicates the standard deviation of  $\delta$ .

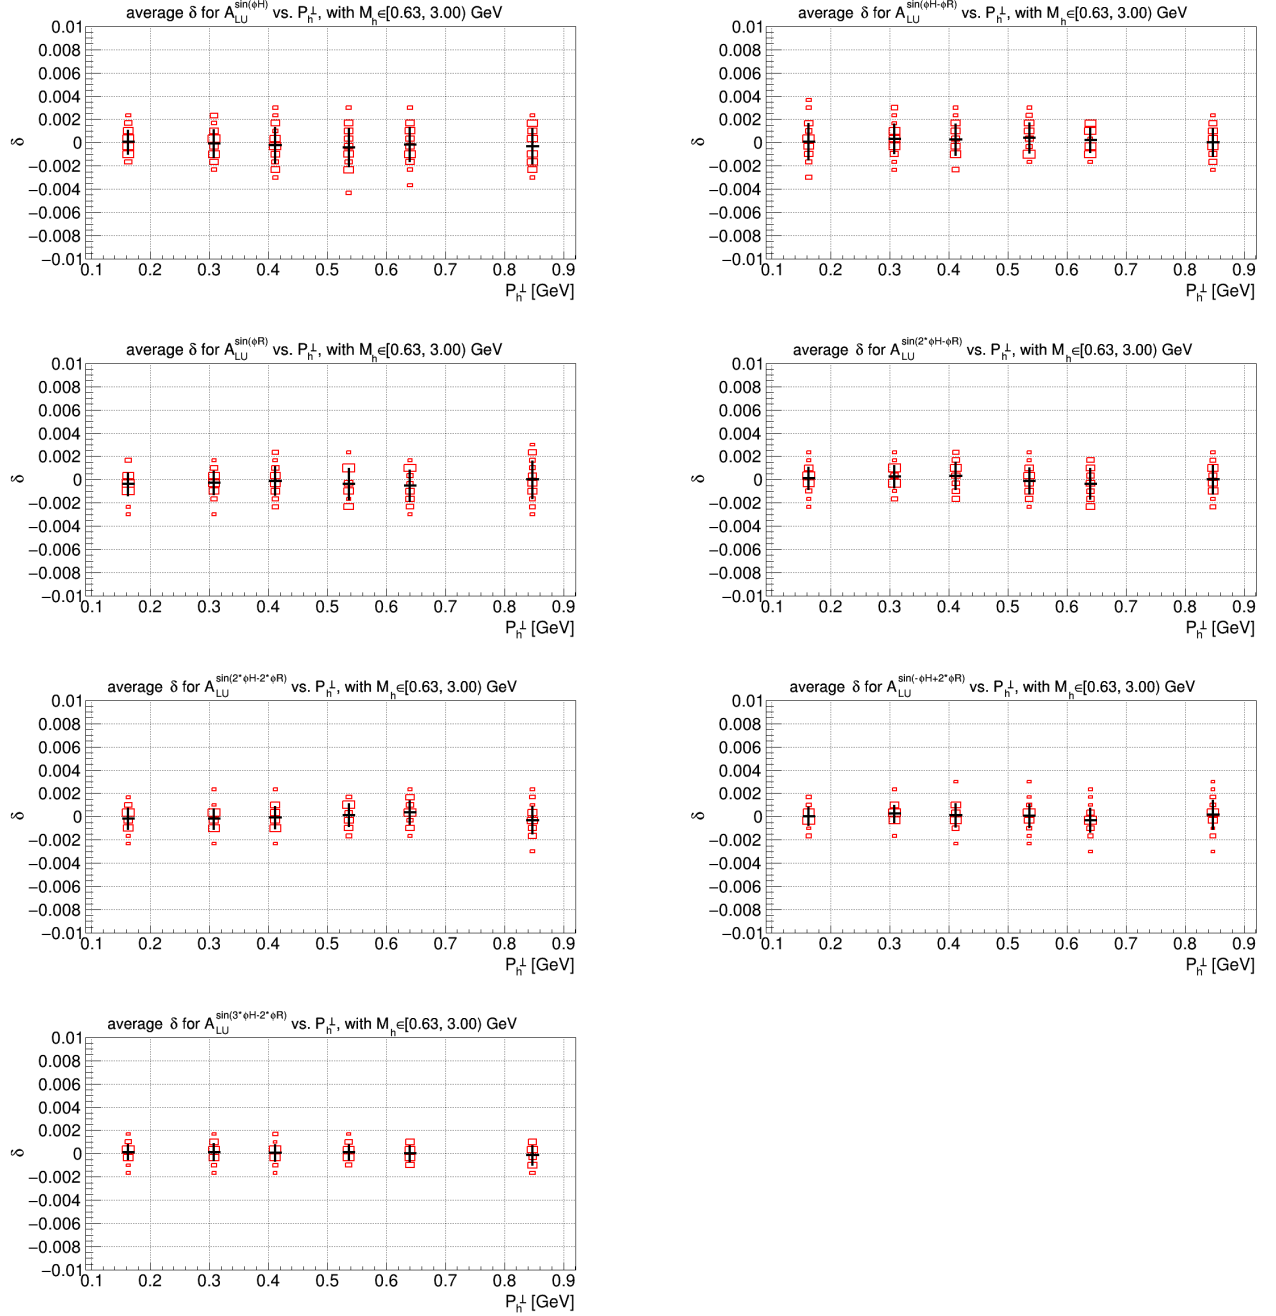

FIG. 10: Distribution of  $\delta$  for each kinematic bin and  $\sigma_{LU}$  modulation; this is for the binning in  $P_h^\perp$ , with  $M_h > 0.63$  GeV. One histogram entry (red box plot) corresponds to one  $\sigma_{UU}$  amplitude injection; the size of the red box is proportional to the number of entries in that bin. The black crosses indicate the mean  $\delta$  for each kinematic bin, and the vertical size of the black cross indicates the standard deviation of  $\delta$ .

#### IV. CORRECTING FOR THE $P_{2,0}$ MODULATION OF THE UNPOLARIZED CROSS SECTION

The full partial wave expansion of the dihadron cross section also includes modulations in  $\theta$ , the dihadron frame decay angle. The modulation  $P_{2,0}(\cos\theta) = (3\cos^2\theta - 1)/2$  of  $d\sigma_{UU}$  is of particular importance and has been studied in other measurements, such as those from HERMES [4], where they employed a similar strategy as our aforementioned Monte Carlo study. Since this modulation is dependent only on  $\theta$  and not on  $\phi_h$  or  $\phi_{R\perp}$ , we find the shift  $\delta$  on  $A_{LU}$  to be

$$\delta = \frac{AB\langle P_{2,0} \rangle}{1 + B\langle P_{2,0} \rangle}, \quad (6)$$

where  $A$  is the original  $A_{LU}$  amplitude,  $B$  is the amplitude of  $P_{2,0}$ , and  $\langle P_{2,0} \rangle$  is the mean value of  $P_{2,0}$  from the data. Tables XV-XX give the value of  $\langle P_{2,0} \rangle$  for each kinematic bin used in the asymmetry analysis. When a proper measurement of the amplitude of this modulation becomes available, Eq. 6 can be used in combination with the values listed in these tables in order to correct the presented  $A_{LU}$  values.

| Bin | $\langle x \rangle$ | $\langle P_{2,0}(\cos \theta) \rangle$ |
|-----|---------------------|----------------------------------------|
| 1   | 0.105               | -0.404                                 |
| 2   | 0.127               | -0.408                                 |
| 3   | 0.143               | -0.410                                 |
| 4   | 0.157               | -0.412                                 |
| 5   | 0.174               | -0.414                                 |
| 6   | 0.191               | -0.417                                 |
| 7   | 0.211               | -0.418                                 |
| 8   | 0.235               | -0.419                                 |
| 9   | 0.261               | -0.419                                 |
| 10  | 0.294               | -0.419                                 |
| 11  | 0.342               | -0.419                                 |
| 12  | 0.441               | -0.419                                 |

TABLE XV: Mean values of  $P_{2,0}(\cos \theta)$  for the binning scheme in  $x$ .

| Bin | $\langle M_h \rangle$ (GeV) | $\langle P_{2,0}(\cos \theta) \rangle$ |
|-----|-----------------------------|----------------------------------------|
| 1   | 0.338                       | -0.338                                 |
| 2   | 0.422                       | -0.409                                 |
| 3   | 0.496                       | -0.420                                 |
| 4   | 0.568                       | -0.426                                 |
| 5   | 0.641                       | -0.428                                 |
| 6   | 0.708                       | -0.429                                 |
| 7   | 0.759                       | -0.427                                 |
| 8   | 0.805                       | -0.426                                 |
| 9   | 0.864                       | -0.425                                 |
| 10  | 0.939                       | -0.422                                 |
| 11  | 1.045                       | -0.417                                 |
| 12  | 1.271                       | -0.404                                 |

TABLE XVI: Mean values of  $P_{2,0}(\cos \theta)$  for the binning scheme in  $M_h$ .

| Bin | $\langle z \rangle$ | $\langle P_{2,0}(\cos \theta) \rangle$ |
|-----|---------------------|----------------------------------------|
| 1   | 0.400               | -0.461                                 |
| 2   | 0.474               | -0.430                                 |
| 3   | 0.528               | -0.409                                 |
| 4   | 0.579               | -0.390                                 |
| 5   | 0.638               | -0.368                                 |
| 6   | 0.727               | -0.325                                 |

TABLE XVII: Mean values of  $P_{2,0}(\cos \theta)$  for the binning scheme in  $z$ , with  $M_h < 0.63$  GeV.

| Bin | $\langle z \rangle$ | $\langle P_{2,0}(\cos \theta) \rangle$ |
|-----|---------------------|----------------------------------------|
| 1   | 0.404               | -0.477                                 |
| 2   | 0.474               | -0.456                                 |
| 3   | 0.528               | -0.440                                 |
| 4   | 0.580               | -0.424                                 |
| 5   | 0.638               | -0.403                                 |
| 6   | 0.731               | -0.354                                 |

TABLE XVIII: Mean values of  $P_{2,0}(\cos \theta)$  for the binning scheme in  $z$ , with  $M_h > 0.63$  GeV.

| Bin | $\langle P_h^\perp \rangle$ (GeV) | $\langle P_{2,0}(\cos \theta) \rangle$ |
|-----|-----------------------------------|----------------------------------------|
| 1   | 0.169                             | -0.427                                 |
| 2   | 0.311                             | -0.420                                 |
| 3   | 0.426                             | -0.414                                 |
| 4   | 0.533                             | -0.408                                 |
| 5   | 0.653                             | -0.400                                 |
| 6   | 0.863                             | -0.379                                 |

TABLE XIX: Mean values of  $P_{2,0}(\cos \theta)$  for the binning scheme in  $P_h^\perp$ , with  $M_h < 0.63$  GeV.

| Bin | $\langle P_h^\perp \rangle$ (GeV) | $\langle P_{2,0}(\cos \theta) \rangle$ |
|-----|-----------------------------------|----------------------------------------|
| 1   | 0.160                             | -0.434                                 |
| 2   | 0.306                             | -0.428                                 |
| 3   | 0.422                             | -0.424                                 |
| 4   | 0.530                             | -0.418                                 |
| 5   | 0.648                             | -0.413                                 |
| 6   | 0.852                             | -0.402                                 |

TABLE XX: Mean values of  $P_{2,0}(\cos \theta)$  for the binning scheme in  $P_h^\perp$ , with  $M_h > 0.63$  GeV.

- 
- [1] A. Bacchetta and M. Radici, Phys. Rev. D **67**, 094002 (2003), arXiv:hep-ph/0212300.
  - [2] A. Bacchetta and M. Radici, Phys. Rev. D **69**, 074026 (2004), arXiv:hep-ph/0311173.
  - [3] S. Gliske, A. Bacchetta, and M. Radici, Phys. Rev. D **90**, 114027 (2014), [Erratum: Phys.Rev.D 91, 019902 (2015)], arXiv:1408.5721 [hep-ph].
  - [4] A. Airapetian *et al.* (HERMES Collaboration), JHEP **06**, 017 (2008), arXiv:0803.2367 [hep-ex].
